# Supplementary material for: GaussTR: Foundation Model-Aligned Gaussian Transformer for Self-Supervised 3D Spatial Understanding
Source: arXiv:2412.13193 source file (2025-03-24)
Supplement: Supplementary file 1 [file X_suppl.tex]

\clearpage
\setcounter{page}{1}

\maketitlesupplementary

\begin{figure}
    \centering
    \includegraphics[width=\textwidth]{fig/4_additional_visualization.pdf}
    \caption{\textbf{Additional Visualizations from camera views.}}
    \label{fig:add_vis}
\end{figure}

\section{Additional Visualizations}
As shown in \cref{fig:add_vis}, we provide visualizations of the rendered depth and semantic maps projected onto camera views. To enhance interpretability, we introduce color perturbations to the semantic maps, highlighting the distribution of individual Gaussians and offering insights into how they collectively form the scene layout.
Additionally, we demonstrate GaussTR's ability to generalize to novel and scarce categories, such as traffic lights and street signs. Thanks to its alignment with foundation models, GaussTR seamlessly transfers to these categories, producing prominent activations in the corresponding regions, as highlighted by the red boxes.
